# Supplementary material for: Multi-step planning with learned effects of partial action executions
Source: arXiv:2303.09355 source file (2023-11-17)
Supplement: Supplementary file 1 [file additional.tex]

\begingroup
\begin{table}[thbp]
\tbl{n-step prediction errors, results from our experiments.}
{\begin{tabular}{|c|c|c|} \hline
 & \textbf{Sp-Truth}& \textbf{Im-CNN}\\\hline
\textbf{1-step (cm)} & $0.354 \pm 0.072$ & $0.340 \pm 0.044$ \\\hline
\textbf{2-step (cm)} & $0.390 \pm 0.061$  & $0.352 \pm 0.046$ \\\hline
\textbf{3-step (cm)} & $0.417 \pm 0.053$  & $0.364 \pm 0.049$ \\\hline
\textbf{4-step (cm)} & $0.445 \pm 0.046$  & $0.375 \pm 0.051$ \\\hline
\textbf{5-step (cm)} & $0.474 \pm 0.039$  & $0.387 \pm 0.054$ \\\hline
\end{tabular}}
\label{table:cnmp_n_step_errors}
\end{table}
\endgroup
